# Supplementary material for: Yielding behavior of glasses under asymmetric cyclic deformation
Source: arXiv:2201.06535 ancillary file (2022-01-19)
Supplement: Supplementary file 1 [file Onesidedshear_SM.pdf]

# Yielding behavior of glasses under asymmetric cyclic deformation (Supplemental Material)

Monoj Adhikari,[1] Muhittin Mungan,[2] and Srikanth Sastry[1,*]

[1]*Jawaharlal Nehru Centre for Advanced Scientific Research, Jakkar Campus, 560064 Bengaluru, India*
[2]*Institut für angewandte Mathematik, Universität Bonn, Endenicher Allee 60, 53115 Bonn, Germany*

## S1. DESCRIPTION OF THE MODEL AND DEFORMATION PROTOCOL

We describe below the model system we study in this work, and provide details of the investigations we carry out computationally. We study the Kob-Andersen binary Lennard-Jones mixture (KA-BMLJ) whose interactions are given by

$$V_{\alpha\beta}(r) = \begin{cases} 4\epsilon_{\alpha\beta}\left(\left(\frac{\sigma_{\alpha\beta}}{r}\right)^{12} - \left(\frac{\sigma_{\alpha\beta}}{r}\right)^{6}\right) - 4\epsilon_{\alpha\beta}\left(c_0 + c_2\left(\frac{r}{\sigma_{\alpha\beta}}\right)^2\right), & r_{\alpha\beta} \leq r_{c,\alpha\beta}, \\ 0, & r_{\alpha\beta} > r_{c,\alpha\beta} \end{cases} \tag{S1}$$

where $\alpha, \beta \in$ {A,B}, $\epsilon_{AB}/\epsilon_{AA} = \epsilon_{BA}/\epsilon_{AA} = 1.5$, $\epsilon_{BB}/\ \epsilon_{AA} = 0.5$, and $\sigma_{AB}/\sigma_{AA} = \sigma_{BA}/\sigma_{AA} = 0.8$, $\sigma_{BB}/\sigma_{AA} = 0.88$. The interaction potential has cut off, $r_{c,\alpha\beta} = 2.5\sigma_{\alpha\beta}$. We report results in reduced units, with units of length, energy and time scales being $\sigma_{AA}$, $\epsilon_{AA}$ and $\sqrt{\frac{\sigma_{AA}^2 m_{AA}}{\epsilon_{AA}}}$ respectively. We simulate samples consisting of $N = 200, 400, 800, 4000, 8000, 32000, 64000$ particles in three dimensions. The system, at fixed number density ($N/V$, $V$ being the volume) $\rho = 1.2$ is equilibrated at reduced temperature $T = 1.0, 0.60, 0.466, 0.40, 0.37$ *via* a constant temperature molecular dynamics simulation. Subsequently, equilibrated configurations are subjected to energy minimization to obtain the inherent structure configurations that have energy $E_{init} = -6.89, -6.92, -6.98, -7.03, -7.05$ respectively for those above-mentioned temperatures.

Athermal Quasi-Static (AQS) shear deformations are carried out in two steps: (i) Particles are displaced by applying an affine transformation, $x\prime = x + d\gamma\ z$, where $d\gamma$ is the strain increment in the $xz$ plane, with $y$ and $z$ coordinates unaltered. Shear strain $\gamma$ is incremented by small strain steps ($d\gamma = 2 \times 10^{-4}$) (ii) The energy of the deformed configuration is minimized, subject to Lees- Edwards periodic boundary conditions [1], which are appropriate for shear deformed simulated systems. These two steps, which closely approximate quasi-static, athermal, deformation, are repeated until the configuration at target strain $\gamma^1_{\max}$ is reached. The sign of $d\gamma$ is then reversed until a zero strain is reached. The cycle is then repeated.

## S2. AVERAGE STRESS AND ENERGY VS STRAIN

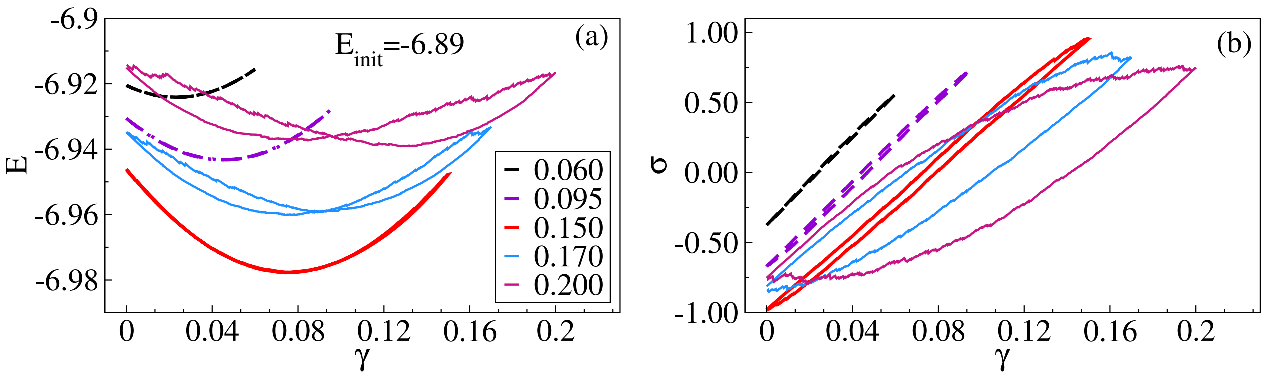


FIG. S1. (a) Energy (averaged over different configurations) against strain $\gamma$ at steady-state and for different asymmetric cyclic shear strain amplitudes $\gamma^1_{\max}$, as indicated in the legend. (b) The corresponding averaged stress values $\sigma$.

* Corresponding author: sastry@jncasr.ac.in

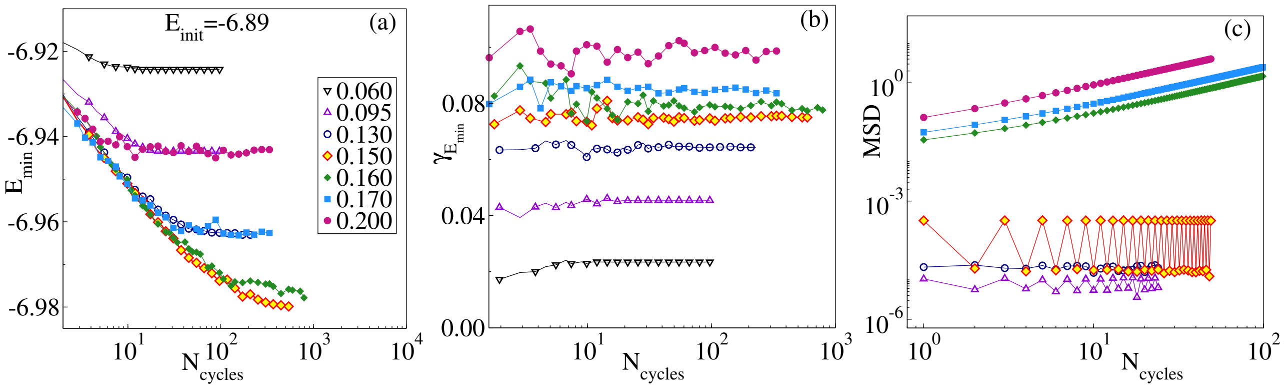


FIG. S2. Poorly-annealed system with initial energy $E_{init} = -6.89$. (a) Evolution of the minimum energy $E_{min}$ attained, (b) plastic strain $\gamma_{E_{min}}$, and (c) mean-squared displacement (MSD) as a function of number $N_{\text{cycles}}$ of training cycles for different strain amplitudes $\gamma^1_{\text{max}}$, as indicated in the legend of (a).

In Fig. S1 (a) and (b) we respectively show the average energy and stress at steady state as a function of $\gamma$, averaged over 15 samples. The corresponding data sets for a single sample are shown in the main text, in Fig. 1. The energy loop becomes open above a strain value of $\gamma^1_{\text{max}} = 0.150$, indicating that the system has reached a diffusive state. Based on the bifurcation of the energy loop we estimate the yielding point to be around $\gamma^1_{max} \sim 0.160$. Similarly, the stress-strain loop also demonstrates that diffusion sets in when $\gamma^1_{max} > 0.150$, as this is the point at which the area of the loop starts to grow. Note that the minimum of the energy occurs at some non-zero strain, which we denote as $\gamma_{E_{min}}$.

## S3. APPROACH TO THE STEADY STATE

In Fig. S2(a), we show, for the poorly-annealed system with initial energy $E_{init} = -6.89$, the evolution of $E_{min}$ against the number of cycles $N_{\text{cycles}}$. We observe that the energy reaches a steady state value after a transient. This steady state value depends upon the amplitude by which it is deformed: the steady state energy decreases until strain amplitude $\gamma^1_{max} = 0.150$, beyond which it starts to increase again, suggesting the onset of yielding around $\gamma_y \sim 0.160$. In Fig. S2(b) we show $\gamma_{E_{min}}$ as a function of the number of cycles $N_{\text{cycles}}$. As the number of cycles $N_{\text{cycles}}$ of shear deformation increases, $\gamma_{E_{min}}$ moves from zero to a non-zero value at which it saturates in the steady state for all amplitudes below yielding. However, above the yielding amplitude, $\gamma_{E_{min}}$ fluctuates around a mean value. Fig. S2 (c) shows the evolution of the mean-squared displacements (MSD) of particles with the number of driving cycles $N_{\text{cycles}}$. For all strain amplitudes $\gamma^1_{\text{max}} < 0.15$, the MSD is almost zero, implying that these states are absorbing states of a cyclic response, whereas the system becomes diffusive starting from the strain amplitude, 0.160. This behavior of MSD clearly demonstrates that the yielding amplitude is around $\gamma_y \sim 0.160$. The corresponding data for the well annealed case is shown in the main text, Fig. 2 (a) - (c).

## S4. SYSTEM SIZE ANALYSIS

In Fig. S3, we show the system size dependence of $\gamma_{E_{min}}$, $E_{min}$, and $\sigma_{max}$, the stress at maximum strain $\gamma^1_{\text{max}}$ for a poorly-annealed glass, $E_{init} = -6.89$, and different system sizes $N$, indicated in the legend of (b). The corresponding data for the well annealed case is shown in the main text, Fig. 4. (a) For system sizes larger than 4000, $E_{\text{min}}$ reaches its lowest value around $\gamma^1_{\text{max}} = 0.15$, which we interpret as the yielding amplitude. Note that this is twice the corresponding value for symmetric shear. (b), The behavior of the plastic strain $\gamma_{E_{min}}$ with $\gamma^1_{\text{max}}$ has almost no dependence on system size and closely follows the line $\gamma_{E_{\text{min}}} = \gamma_{\text{min}}/2$. This is in stark contrasting with the response of the well annealed glasses to asymmetric shear, shown in Fig. 4(b) of the main text. (c) System size dependence of the stress $\sigma_{\text{max}}$ at strain $\gamma^1_{\text{max}}$. With increasing system size $N$ the strain $\gamma^1_{\text{max}}$ at which $\sigma_{max}$ reaches its maximum moves to $\gamma^1_{\text{max}} \approx 0.15$. At the same time, the subsequent stress-drop becomes sharper with increasing $N$.

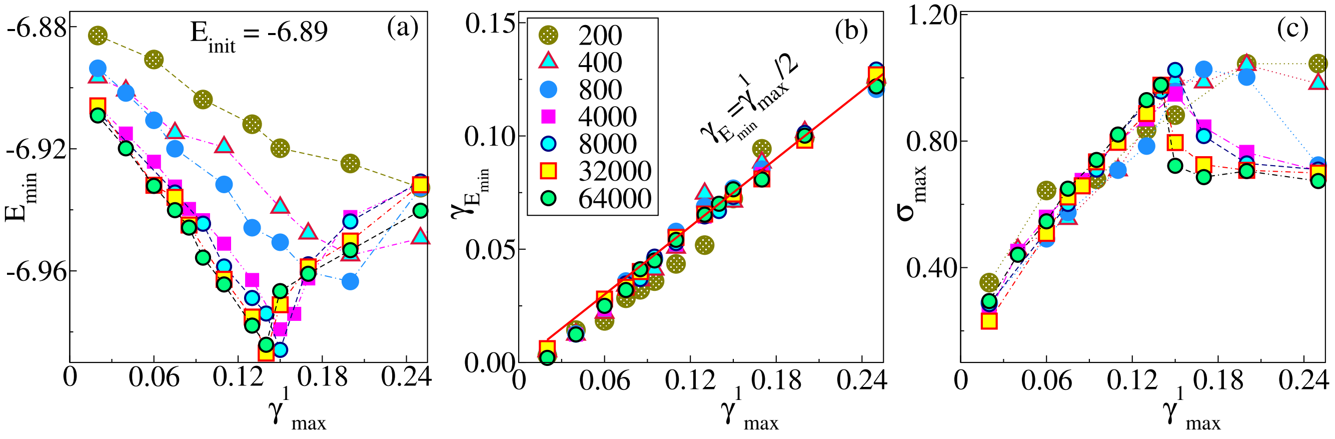


FIG. S3. (a) - (c): System size dependence of $E_{min}$, $\gamma_{E_{min}}$, and $\sigma_{max}$, for a poorly- annealed system with initial energy $E_{init} = -6.89$. The systems sizes $N$ are indicated in (b). The red line in (b) corresponds to $\gamma_{E_{min}} = \gamma^1_{max}/2$.

## S5. LOCATION OF THE STRESS MAXIMUM, $\gamma_{\rm peak}$, AND THE ONSET OF DIFFUSION, $\gamma_{\rm diff}$, FOR WELL ANNEALED GLASSES FOR DIFFERENT SYSTEM SIZES

The system size dependence of $E_{\rm min}$, $\gamma_{E_{\rm min}}$ and the maximum stress, $\sigma_{max}$, are shown in the main text, Fig. 4. In Fig. S4 we show again the stress at the maximum strain, as a function of the maximum strain $\gamma^1$max (Left panel) and the $MSD$ as a function of the number of cycles for different systems sizes of a well-annealed glass with $E_{init} = -7.05$. The left triangle marks the value of the amplitude of asymmetric strain $\gamma_{\rm diff}$ from which diffusive behavior sets in. The values of $\gamma_{\rm diff}$ extracted from the $MSD$ vs. $N_{cycles}$ plots are: 0.160, 0.150 0.130 and 0.120 for the system sizes 4000, 8000, 32000 and 64000 respectively. These plots clearly demonstrate that with increasing system sizes the difference between $\gamma_{\rm peak} = 0.095$ and $\gamma_{\rm diff}$ decreases.

## S6. TWO DIMENSIONAL PAIR CORRELATION FUNCTION, $g_{\rm AA}(x, z)$

We compute the two dimensional directional pair correlation function $g_{\rm AA}(x, z)$ in the shear plane $xz$, which is defined as:

$$g_{\rm AA}(x, z) = \frac{1}{2N\rho} \left\langle \sum_{i=1}^{N-1} \sum_{j\neq i}^{N} \delta(x - (x_i - x_j))\delta(z - (z_i - z_j))\theta(a - |y_i - y_j|), \right\rangle \tag{S2}$$

where $\langle .. \rangle$ denotes averaging over independent samples, and $x_i, y_i, z_i$ are the coordinates of the A particles. Since we compute a two dimensional correlation function in a three dimensional system, we consider pairs of particles with are in the same (shear) plane, by demanding that their vertical ($y$) separations do not exceed a specified value $a = 0.02\sigma_{AA}$. This is enforced by the Heaviside function $\theta(a - |y_i - y_j|)$. In practice, we divide the simulation box into slabs of fixed width $a$ along the $y$ direction and compute $g(x, z)$ for pairs of particles within each slab, averaging over all the slabs.

We compute $g_{\rm AA}(x, z)$ for poorly annealed system as well annealed systems in the steady state. In the top row of Fig. S5 we show the results for a poorly annealed system ($E_{init} = -6.89$), for the values of $\gamma^1_{\rm max} = 0.130, 1.150, 0.170$, which are below, near and above yielding. In all three cases the steady-state particle configuration at zero strain value are used. Although the system has been driven with asymmetric cyclic shear deformations, $g_{\rm AA}(x, z)$ shows nevertheless for all three values of $\gamma^1_{\rm max}$ isotropic behaviour, very similar to what one observes in a liquid structure. In the bottom row Fig. S5 we show $g_{\rm AA}(x, z)$ for a well annealed glass ($E_{init} = -7.05$) and at the same values asymmetric cyclic shear amplitudes $\gamma^1_{\rm max} = 0.130, 1.150, 0.170$, which again correspond to the values below, near and above yielding, *cf.* top row of Fig. S4. As in the poorly annealed case $g_{\rm AA}(x, z)$ is isotropic, and hence the annealing does not introduce any structural changes.

[1] A W Lees and S F Edwards, "The computer study of transport processes under extreme conditions," Journal of Physics C: Solid State Physics **5**, 1921 (1972).

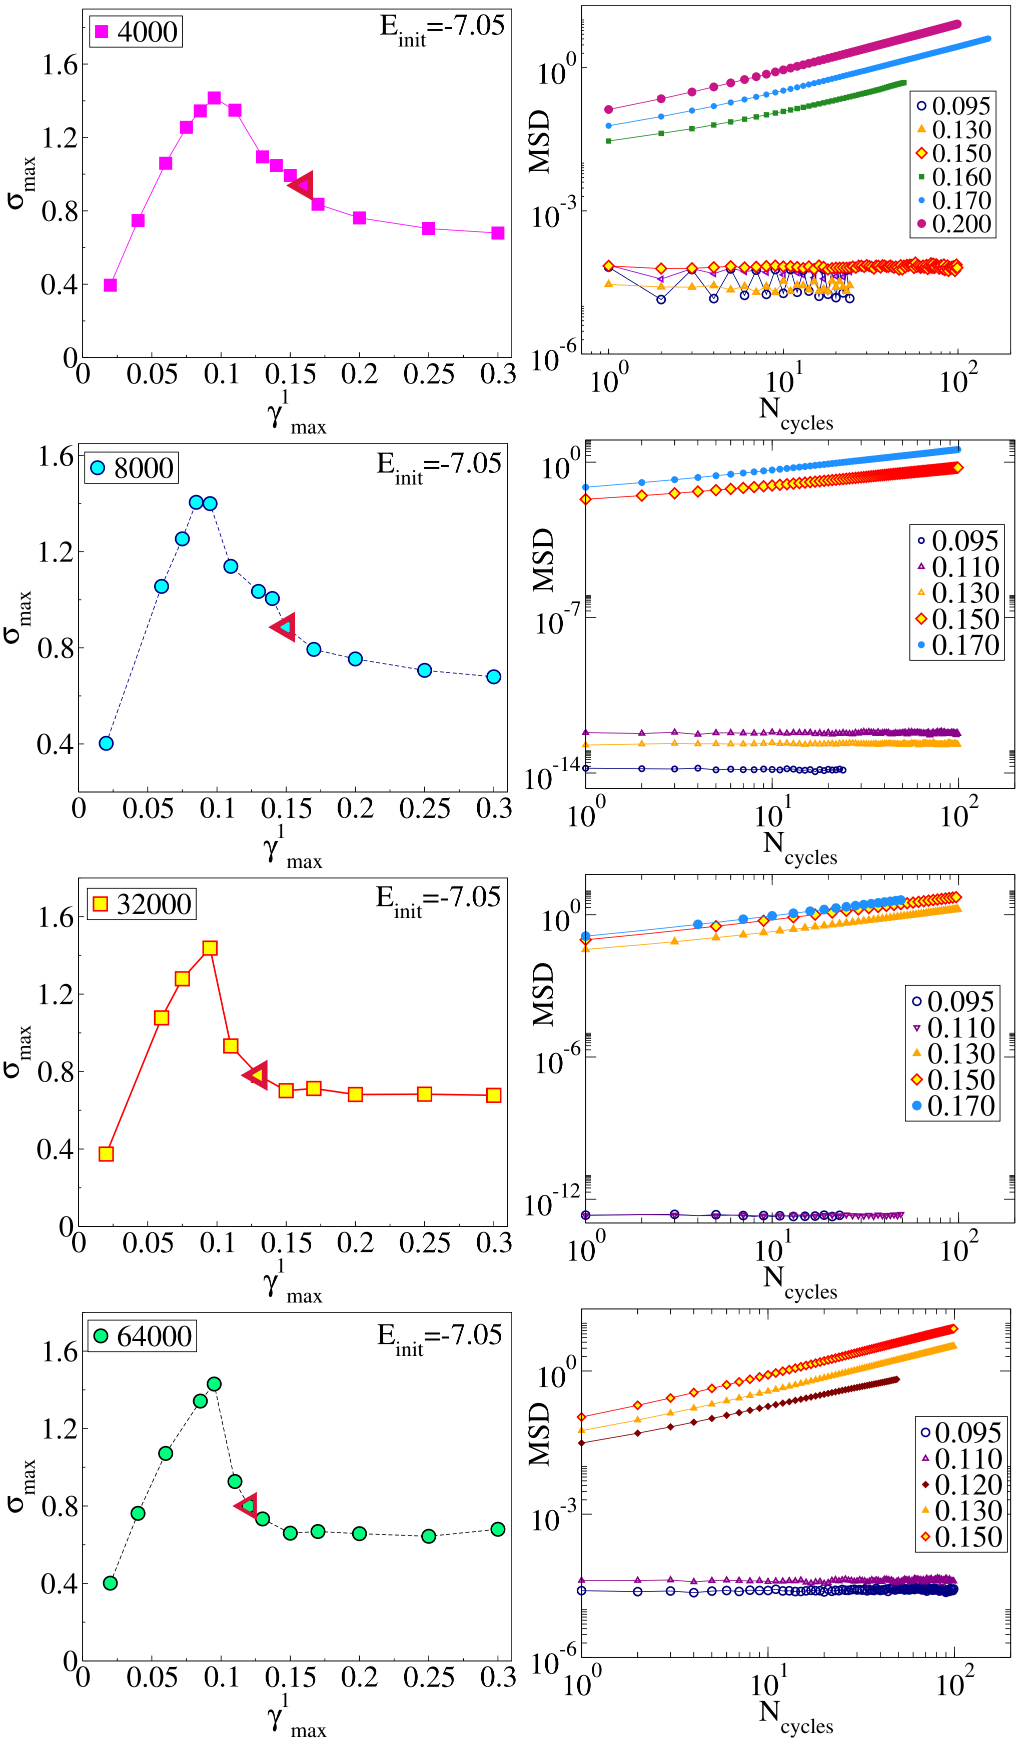


FIG. S4. Left column: Stress is plotted as a function of $\gamma^1_{max}$. Open red triangles correspond to the value of the amplitude of asymmetric strain $\gamma_{\rm diff}$ beyond which diffusive behavior sets in. Right column: The mean squared displacement (MSD) (at the steady state) is plotted against the number of cycles for different $\gamma^1_{max}$.

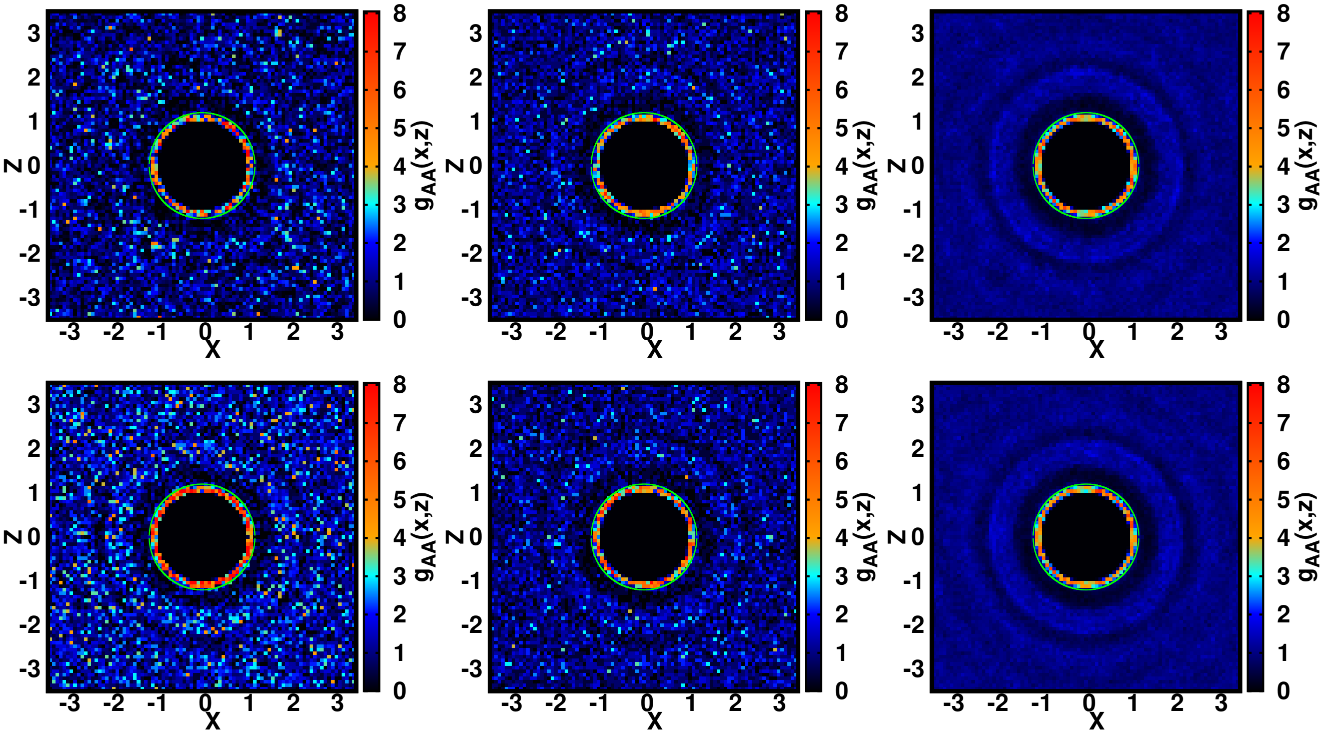


FIG. S5. Two-dimensional pair correlation function $g_{\mathrm{AA}}(x, z)$ computed by considering only the A particles. Top row: poorly annealed glass with $E_{init} = -6.89$ at steady-state reached under asymmetric cyclic shear deformations at $\gamma^1_{\max} = 0.130, 0.150$, and 0.170, corresponding to values (from left to right) below, near, and above yielding respectively. Bottom row: well annealed glass with $E_{init} = -7.05$ and for the same values of asymmetric shear amplitudes $\gamma^1_{\max}$, corresponding to values below, near , and above yielding. The pair correlation functions were obtained by averaging over many cycles in the steady state as well as independent configurations.
